# Supplementary material for: Unconventional anisotropic even-denominator fractional quantum Hall state in a system with mass anisotropy
Source: arXiv:1811.07094 ancillary file (2018-11-17)
Supplement: Supplementary file 1 [file Supplemental_Material.pdf]

# Supplemental Material to "Unconventional anisotropic even-denominator fractional quantum Hall state in a System with mass anisotropy"

Md. Shafayat Hossain, Meng K. Ma, Y. J. Chung, L. N. Pfeiffer, K. W. West, K. W. Baldwin, and M. Shayegan
*Department of Electrical Engineering, Princeton University, Princeton, New Jersey 08544, USA*

(Dated: October 4, 2018)

## I. MATERIALS AND METHODS

Our sample is grown via molecular beam epitaxy on a GaAs substrate. It contains a 20-nm-wide AlAs quantum well (QW) sandwiched by 60-nm $Al_{0.33}Ga_{0.67}$ barriers (Fig. S1). Similar to the case of GaAs, as long as the conduction band offset between the barrier and the QW is sufficiently large, it is possible to confine carriers in the AlAs QW through modulation doping [1–4]. The main difference is that in AlAs the conduction band has lower energy at the X-points of the Brillouin zone instead of the Γ-point. Therefore, the electrons in our AlAs QW are confined in the X-point valleys. Our AlAs QW has a density of $\simeq 3.2 \times 10^{11}$ cm$^{-2}$ with a low-temperature mobility of $1.6 \times 10^6$ cm$^2$/Vs. Details of the growth of such very high quality AlAs 2D electron system (2DES) can be found in Ref. [4].

In bulk AlAs electrons occupy three energetically degenerate ellipsoidal (or six half ellipsoidal) conduction band valleys at the six equivalent X-points of the first Brillouin zone [2]. We denote these valleys as X, Y, and Z with the major axes lying along [100], [010], and [001], respectively (see Fig. S2(a)). The electrons in each valley possess an anisotropic Fermi surface with longitudinal and transverse effective masses of $m_l$ = 1.0 and $m_t = 0.20$ in units of the free electron mass.

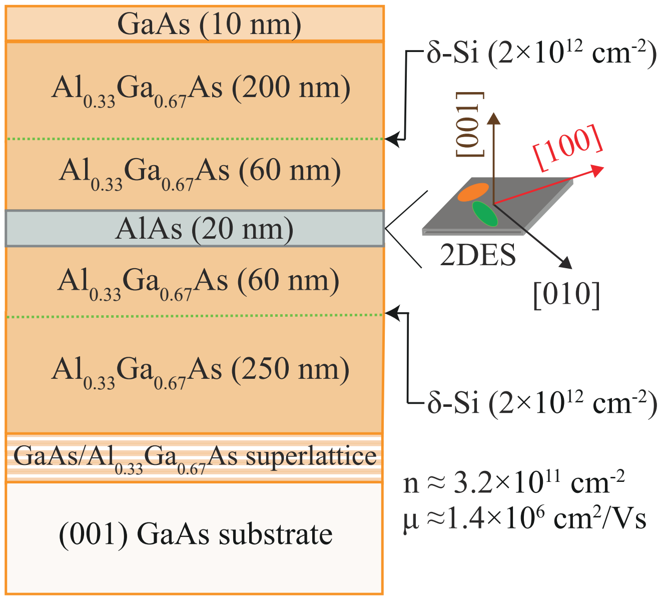


FIG. S1. Structure of our AlAs 2DES grown on a GaAs substrate. The growth direction is [001]. The AlAs layer is under compressive biaxial strain because of the slightly larger lattice constant of AlAs relative to GaAs. This strain results in the occupancy of X and Y valleys only.

When an AlAs QW is formed along the [001] axis, the confinement in the growth direction splits the three-fold valley degeneracy because of the difference in the effective mass along the in-plane and out-of-plane directions. We refer to the out-of-plane valley as Z, and the in-plane valleys as X and Y. At first sight, one would expect that the Z valley should be occupied at all well widths, since it has the larger confinement mass. However, the slightly larger lattice constant of AlAs compared to GaAs causes biaxial compression in the plane of the AlAs layer, lowering the conduction band of the X and Y valleys relative to the Z valley. This causes the ground-state energies of the two types of valleys to cross at a critical QW width of $\simeq 6$ nm [2]. Above this well-width, the X and Y valleys are occupied; this is the case for our 20-nm-wide AlAs QW (Figs. S1 and S2(b)).

In the absence of any additional in-plane strain, electrons in our AlAs QW occupy two in-plane valleys (X and Y). This two-fold valley-degeneracy can be lifted via the application of an in-plane, symmetry-breaking, strain $\varepsilon = \varepsilon_{[100]} - \varepsilon_{[010]}$, where $\varepsilon_{[100]}$ and $\varepsilon_{[010]}$ are the strain values along [100] and [010] [2]. The valley splitting energy is given by $E_V = \varepsilon E_2$, where $E_2$ is the deformation potential, which in AlAs has a band value of 5.8 eV. Positive strain pushes the energy of the X valley up relative to the Y valley, causing electrons to transfer from X to Y, and vice versa for negative strain.

In Fig. S2(c) we show our experimental setup for applying tunable in-plane strain to the 2DES. We glue the sample on one side of a stacked piezo-electric lead-zirconate-titanate (PZT) actuator with a commercial two-part epoxy [5]. The piezo-electric actuator deforms when a voltage ($V_P$) is applied across its two leads and hence strains the sample glued on top of it. Thus, we introduce nearly uniaxial, in-plane strain to our 2DES. The amount of strain can be measured by a strain gauge glued on the back-side of the piezo-electric actuator (Fig. S2(c)). We find the strain to be $3.6 \times 10^{-7}$ per Volt applied to the piezo-actuator.

In order to maintain sufficient strain homogeneity, we used small van der Pauw samples with typical dimensions of 1.5 mm ×1.5 mm. Note that the sample edges are along the GaAs cleave directions, [110] and [$\bar{1}$10] (see

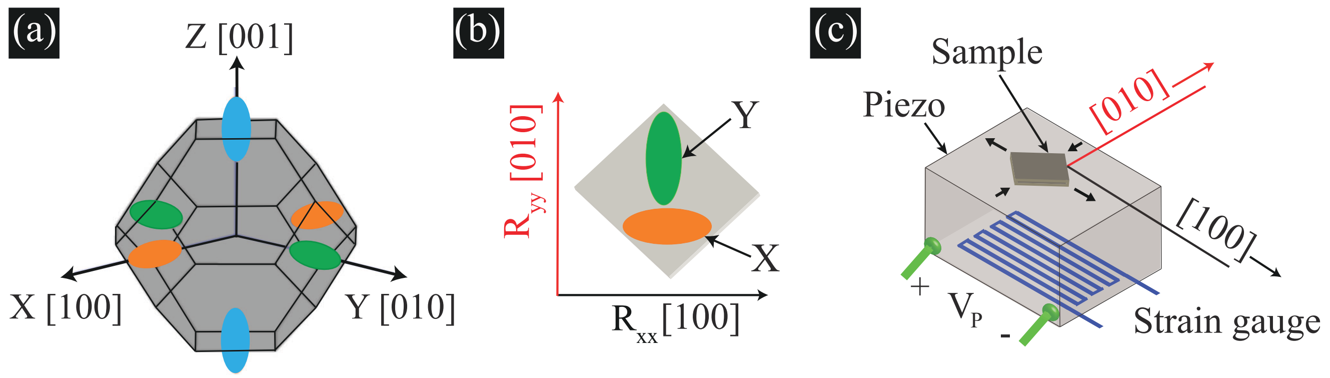


FIG. S2. (a) First Brillouin zone and constant energy surfaces of the lowest energy bands for bulk AlAs, showing the X, Y, and Z valleys; [100] and [010] refer to the crystallographic directions. (b) The sample geometry, including the orientation of the two occupied valleys (X and Y) and the measured longitudinal resistances ($R_{xx}$ and $R_{yy}$) are shown. (c) Schematic of the experimental setup for applying in-plane strain ($\varepsilon$). The sample and a strain gauge are glued to the opposite sides of a piezo-actuator, and strain is introduced when a bias voltage ($V_P$) is applied to the actuator's leads.

Fig. S2(b)). The samples are lapped and polished on the back-side down to 150 $\mu$m in order for the strain to propagate to the 2DES [5]. Electron-beam evaporated Ti-Au alloy on the back side of the sample shields the 2DES from the electric field generated by the applied $V_P$.

In Fig. S3 we show the voltage and current leads for all the configurations used in our magneto-transport measurements. We carried out our experiments mostly in a dilution refrigerator with a mixing chamber temperature of $T \simeq 0.02$ K and using an 18 T superconducting magnet at the National High Magnetic Field Laboratory (NHMFL), Tallahassee, Florida. The very high field data shown in Fig. S10 were taken in a dilution refrigerator with a mixing chamber temperature of $T \simeq 0.05$ K, equipped with a 45 T hybrid magnet, also located at the NHMFL. The data shown in Figs. S4 and S5 were taken in a $^3$He cryostat with a base temperature of $T \simeq 0.3$ K.

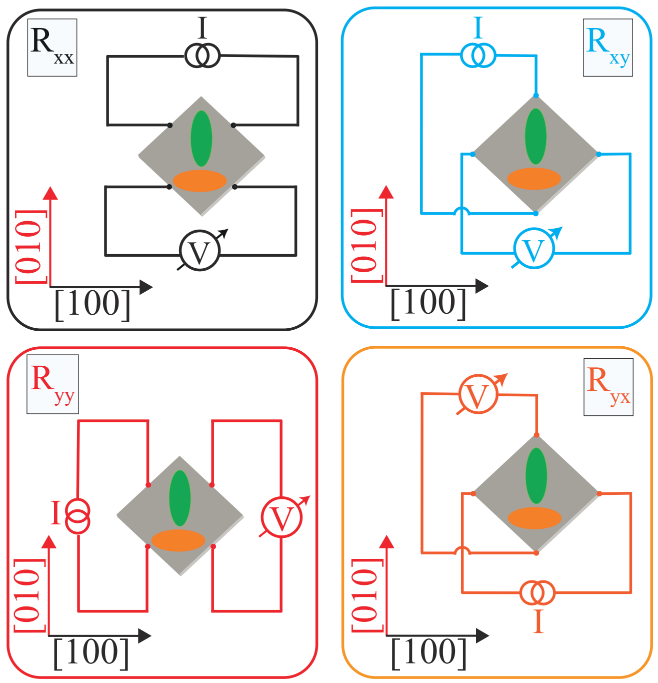


FIG. S3. Configurations showing the current injection and voltage probes used to measure $R_{xx}$, $R_{yy}$, $R_{xy}$, and $R_{yx}$.

## II. MEASUREMENTS OF SPIN SUSCEPTIBILITY

The *band* effective mass for our AlAs 2DES is $m_b = (m_l m_t)^{1/2} = 0.45$ in units of free electron mass, and the effective *band* Landé $g$-factor of AlAs is $g_b = 2$. Note that both the effective mass and $g$-factor are much larger in AlAs than GaAs which has $m_b = 0.067$ and $|g_b| = 0.44$. Moreover, the larger $m_b$, combined with a smaller dielectric constant in AlAs ($\kappa = 10$ compared to 13 for GaAs), renders the AlAs 2DES *effectively* very dilute. Indeed, the parameter $r_s$, the average inter-electron spacing measured in units of the effective Bohr radius, is $\simeq 8.5$ for our sample. Such diluteness means that the electron-electron interaction is strong in our 2DES, which in turn leads to a strong enhancement of the spin susceptibility or, equivalently, a larger value of $g^*m^*/g_b m_b$, where $g^*$ and $m^*$ are the interaction-enhanced effective mass and $g$-factor, respectively [2]. We carried out coincidence measurements to determine $g^*m^*$ for our single-valley AlAs 2DES.

In order to perform the coincidence measurements, the sample glued on the piezo-actuator is mounted on a stage which can be rotated at low temperatures *in situ*. Since the cyclotron energy, $E_C = \hbar e B_\perp / m^*$, depends on the perpendicular field ($B_\perp$) whereas the Zeeman energy, $E_Z = g^* \mu_B B$, depends on the total field ($B$), the Landau levels (LLs) of different orbital indices cross as the sample

is tilted (Fig. S4(a)). Quantitatively, the crossings occur at angles $\theta_j$ according to the expression $E_Z/E_C = j$ or $g^*m^*/2m_0 = j cos(\theta_j)$, where $j$ = 1, 2, 3, ..., and $m_0$ is the free electron mass [6]. As highlighted in the LL diagram in Fig. S4(a), the energy gaps of integer quantum Hall states (IQHSs) oscillate as a function of $1/cos(\theta)$. This leads to oscillations in the resistance for a given IQHS minimum as demonstrated in Fig. S4(b). From the observed period of the oscillations ($\Delta(1/cos(\theta))$), using the relation $g^*m^*/m_0 = 4/\Delta(1/cos(\theta))$, we obtain $g^*m^*/m_0 = 2.70$. Such a large spin susceptibility leads to a value of 1.35 for the ratio of $E_Z$ to $E_C$ in a purely perpendicular magnetic field, and thus results in the LL diagram shown in Fig. S4(a).

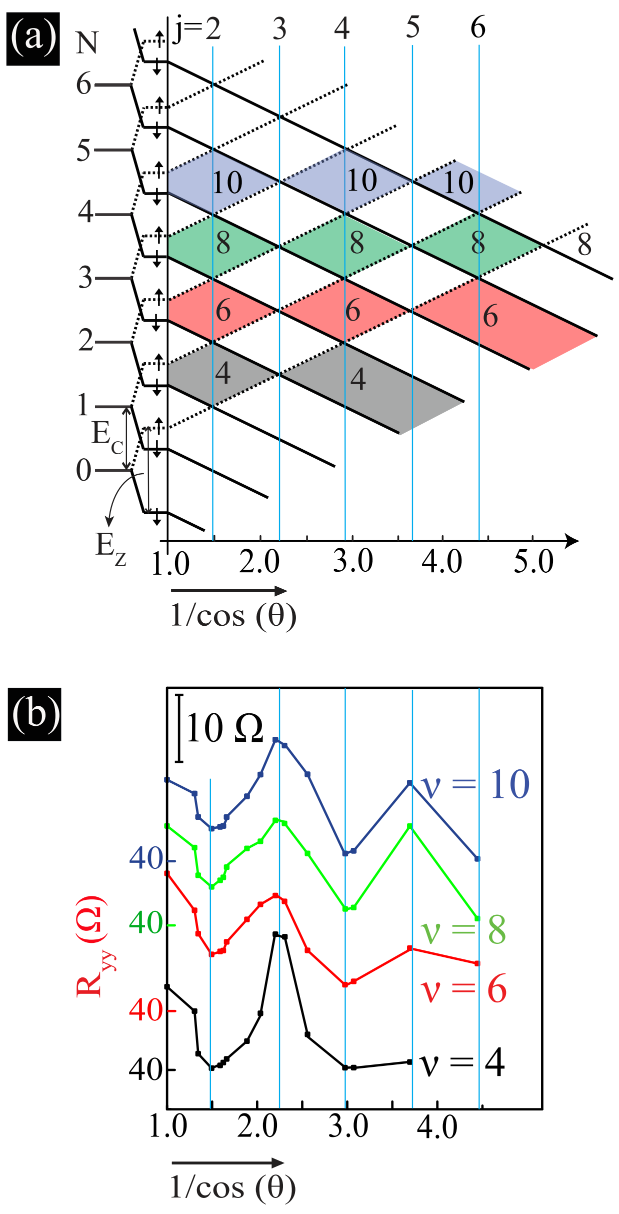


FIG. S4. Determination of spin susceptibility from coincidence measurements. (a) Checkerboard LL diagram showing the LL crossings. Black, red, green, and blue diamonds correspond to the energy gaps of even IQHSs as marked. (b) Measured resistance ($R_{yy}$) at filling factors $\nu$ = 4, 6, 8, and 10 plotted against 1/cos($\theta$), exhibiting clear oscillations. Blue perpendicular lines denote the tilt-angles where the LLs of two opposite spins cross.

It is worthwhile noting that, when $E_Z/E_C = j$ assumes odd integer values such as 3, 5, etc., even IQHSs become weaker, and therefore, the corresponding resistance minima manifest local maxima in Fig. S4(b). On the other hand, when $j$ takes even integer values such as 2, 4, 6, etc., the energy gaps for the even IQHSs are largest and we observe local minima in resistances. In Fig. S4, we mark the positions and values of $j$ accordingly.

We add that, the enhancement in the spin susceptibility in our 20-nm-wide AlAs QW, $g^*m^*/g_b m_b = 3.0$, is $\simeq$ 10% smaller than what has been reported for an 11-nm-wide AlAs QW of similar electron density [7]. This is reasonable as the enhancement decreases with increasing electron layer thickness [7]. When both valleys are occupied, $g^*m^*/g_b m_b$ becomes slightly smaller ($\simeq 2.65$) but $E_Z/E_C$ still remains $> 1$ ($\simeq 1.20$); a more detailed description of LLs in the presence of a valley degeneracy is discussed in Section III. However, for simplicity we have shown similar $E_Z/E_C$ for both single- and bi-valley occupancy in Fig. 2.

## III. MEASUREMENTS OF VALLEY SUSCEPTIBILITY

Similar to the tuning of the spin degree of freedom with the in-plane magnetic field, the valley degree of freedom can be tuned via in-plane uniaxial strain, $\varepsilon$. As we apply $\varepsilon$, valley degeneracy is split by $E_V$ ($= \varepsilon E_2$) which increases linearly with strain. $E_2$ is the deformation potential, which in AlAs has a band value of $E_{2b} = 5.8$ eV. Since our AlAs 2DES is *effectively* very dilute ($r_s \simeq 8.5$), strong electron-electron interaction leads to an enhancement of valley susceptibility [7, 8], similar to the enhancement of the spin susceptibility as described in Section II. Indeed, following the analysis of Gunawan *et al.* [8], we can measure this enhanced valley susceptibility as we outline in this section.

The strain-induced valley splitting causes pairs of quantized LLs of the 2DES in $B_\perp$ to cross at the Fermi energy ($E^F$) as shown schematically in the LL fan diagram in Fig. S5(c). In order to track these crossings, we monitor the resistance along the [110] (cleaved edge) direction ($R_{[110]}$) as a function of $\varepsilon$ at fixed values of $B_\perp$ that correspond to filling factors $\nu$ = 4, 6, 8, and 10. For measuring $R_{[110]}$, we use the configuration shown in Fig. S5(a). In contrast to the [100] or [010] directions, transport along [110] is essentially isotropic, and $R_{[110]}$ does not change when the electrons are transferred from one valley to the other. Therefore, the changes in resistance

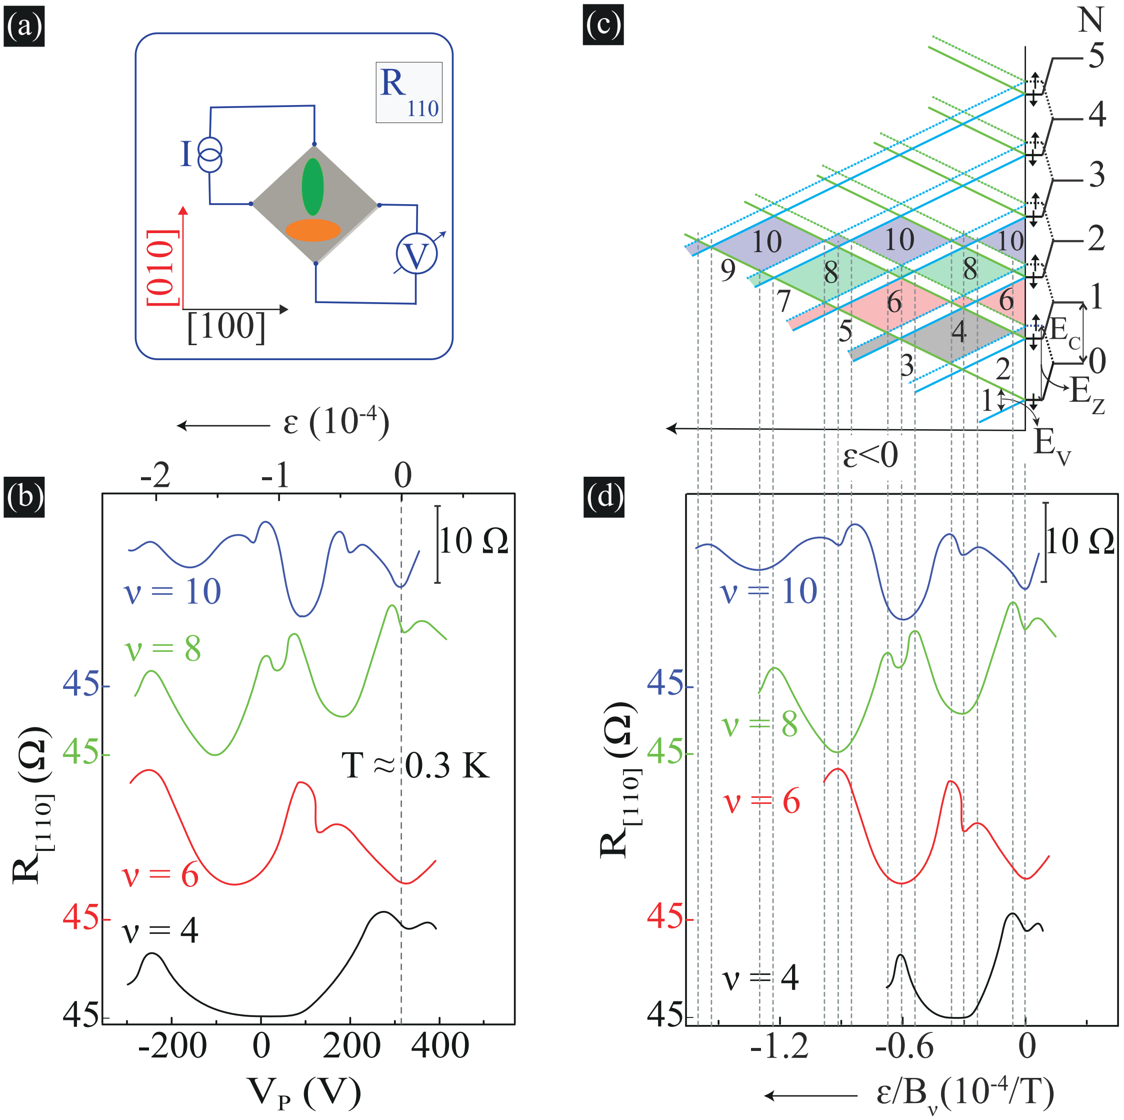


FIG. S5. (a) The configuration we use for measuring $R_{[110]}$. (b) $R_{[110]}$ vs the piezo bias $V_P$ (or strain $\varepsilon$), at various filling factors ($\nu$) measured at $T \simeq 0.35$ K. The traces are vertically offset for clarity. (c) Schematic energy fan diagram showing the relevant energies: the cyclotron ($E_C$), Zeeman ($E_Z$) and valley splitting ($E_V$). (d) Same data as in (b) but now plotted vs a normalized horizontal axis showing that the oscillations have the same period.

of the IQHS minima corresponding to the weakening or strengthening of the energy gap are easily discernible, and free of changes in the background resistance.

We observe clear oscillations in $R_{[110]}$ as a function of piezo-bias, $V_P$ (Fig. S5(b)). The origin of these oscillations can be easily understood from the LL diagram shown in Fig. S5(c). When an integer number of LLs of the 2DES are exactly filled, $E^F$ falls in an energy gap separating adjacent levels and $R_{[110]}$ exhibits a local minimum. However, at certain values of $\varepsilon$, the energy levels corresponding to different valley- and spin-split LLs coincide at $E^F$. At such coincidences, the $R_{[110]}$ minimum becomes weaker. As evident in the fan diagram of Fig. S5(c), the energy gap of an even-integer LL filling oscillates as a function of $\varepsilon$ as $E^F$ falls in a small diamond and a big diamond, one after another. When $E^F$ is inside a gap in a big diamond, $R_{[110]}$ exhibits a strong local minimum. On the other hand, $R_{[110]}$ shows a weak local minimum when $E^F$ is inside a small diamond.

The period of the $R_{[110]}$ oscillations as a function of $\varepsilon$ is larger at smaller $\nu$, i.e. at larger $B_\perp$. In Fig. S5(d) we plot $R_{[110]}$ as a function of $\varepsilon$ normalized by $B_\perp$ [8]. It is clear in this plot that, the oscillations are in-phase at $\nu =$ 4 and 8, and that these are $180^o$ out-of-phase with respect to the oscillations at $\nu = 6$ and 10. From the period of the oscillations, we can calculate the enhancement in the valley susceptibility $E_2^* m^*/E_{2b} m_b = e\hbar/(\Delta\varepsilon/B_\nu)$ where $\Delta\varepsilon$ is the period of oscillations for a given filling factor [8].

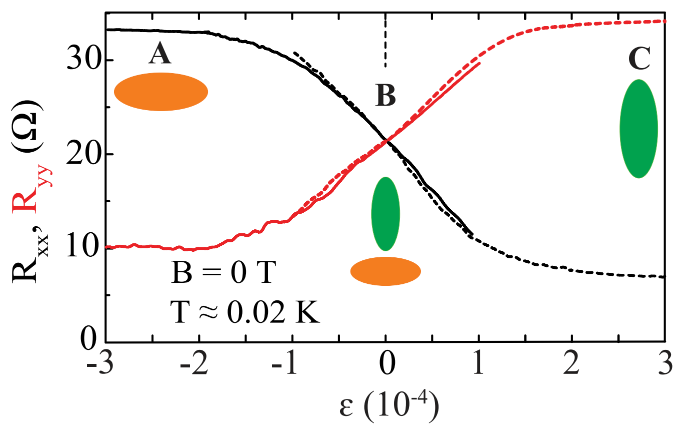


FIG. S6. Sample resistances, $R_{xx}$ (black) and $R_{yy}$ (Red) vs the uniaxial strain $\varepsilon$, measured at $B = 0$ T. Dashed and solid lines represent piezo-resistance traces measured for the two samples that we used to access large positive and negative strains. Resistances represented by the dashed traces are normalized at the balanced point (point **B**) to match with the solid traces.

We find that $E_2^* m^*/E_{2b} m_b \simeq 3.0$ which is consistent with the results of Refs. [7, 8]. Using the valley susceptibility, we can obtain an approximate value of $E_V/E_C$ at $\nu = 3/2$ when $\varepsilon = \pm 3 \times 10^{-4}$; this is $\simeq 2.45$. Such a large $E_V/E_C$ confirms that, at $\varepsilon = \pm 3 \times 10^{-4}$, the electrons are deep in one valley and that $E^F$ at $\nu = 3/2$ is in the $N = 1$ LL.

We would like to remark that, in the presence of a valley degree of freedom, $g^* m^*/g_b m_b$ is expected to decrease slightly [7]. In fact, we can determine the ratio $g^* m^*/g_b m_b$ from Figs. S5(c) and S5(d). It is clear from the LL diagram (Figs. S5(c)) that, the strong and weak minima in $R_{[110]}$ at an even $\nu$ occur at coincidences where $E_V$ is an integer multiple of $E_C$. On the other hand, the local maxima occur when LLs of opposite spin orientations cross, i.e., when $E_V$ equals either $E_Z$ or $jE_C - E_Z$, where $j$ is an integer. For example, at $\nu = 10$, the weak minimum at $\varepsilon/B_\nu = 0.30 \times 10^{-4}$/T happens at the strain position where $E_V/E_C = 1$. The nearby local maximum at $\varepsilon/B_\nu = 0.36 \times 10^{-4}/T$, however, occurs when $E_V/E_Z = 1$. From these values of $\varepsilon/B_\nu$, we obtain $E_Z/E_C = g^* m^*/2m_0$ to be $\simeq 1.20$. Thus, we find $g^* m^*/g_b m_b \simeq 2.65$ for our AlAs QW when electrons occupy both X and Y valleys; this is slightly ($\simeq 10\%$) smaller than the case where electrons in our AlAs QW occupy only one valley (see Section III).

Another noteworthy feature of Fig. S5 data is that, a finite $V_P$ is required to attain the zero-strain condition in our experiments [8]; this is about 315 V for our data shown in Fig. S5 and is marked by a dashed vertical line in Fig. S5(b). Such offset in $\varepsilon$ occurs because of the cooldown- and sample-dependent residual strain originating from the difference in thermal contraction coefficients between the sample, glue and the piezo-actuator during the cooling process [8]. Intriguingly, the data of Fig. S5(b) provide us with an alternative way to determine the zero-strain condition: at $V_P = 315$ V, $R_{[110]}$ at $\nu = 4$ and 8 is at a (local) weak minimum while at $\nu = 6$ and 10, it is at a (local) strong minimum. This behavior is consistent with the LL diagram of Fig. S5(c) when no strain is present ($\varepsilon = 0$).

## IV. EXPERIMENTAL CONSIDERATIONS FOR APPLICATION OF STRAIN

Because of the finite, cooldown- and sample-dependent residual strain as discussed in Section III, we could not reach the two extremes of the valley occupancy in the same sample within the accessible $V_P$ limit. Therefore, in order to reach the regimes where all the electrons occupy only X or only Y valley, we used two different samples. The piezo-resistance traces for these samples are shown in Fig. S6 with solid and dashed lines, respectively. We can apply $-3 \times 10^{-4} < \varepsilon < 1 \times 10^{-4}$ in one sample (solid traces), and $-1 \times 10^{-4} < \varepsilon < 3 \times 10^{-4}$ to the other sample (dashed traces). Both samples have overlapping regimes comprising the balanced point ($\varepsilon = 0$) where $R_{xx} = R_{yy}$. This allows us to normalize the resistances represented by the dashed traces at the balanced point (point **B**) to match with the solid traces. The normalizing factor is $\simeq 1.15$. For simplicity, however, in Fig. 1(b) of the main text, we have represented the complete piezo-resistance traces with solid lines.

## V. EVOLUTION OF MAGNETO-TRANSPORT NEAR $\nu = 3/2$ WITH IN-PLANE STRAIN

Here we discuss the evolution of magneto-transport traces near $\nu = 3/2$ ($2 > \nu > 1$) as we tune the valley occupancy of our AlAs 2DES. In Fig. S7 we show plots of $R_{xx}$, $R_{yy}$, and $R_{xy}$ for eight different values of $\varepsilon$ to capture the evolution. At $\varepsilon \simeq 0$ (Fig. S7(a)), 2D electrons occupy both X and Y valleys and the Fermi energy corresponding to $\nu = 3/2$ ($E^F_{3/2}$) lies in the X0↓ and Y0↓ LLs. $\nu = 3/2$ exhibits an isotropic, compressible composite fermion Fermi sea and $\nu = 5/3$ and 4/3 show well-developed fractional quantum Hall states (FQHSs). With the application of small $\varepsilon$, FQHSs at $\nu = 5/3$ and 4/3 undergo subtle transitions thanks to the crossings of composite fermion LLs of two different valleys (X and Y); this is explained in detail in Refs. [9, 10]. In this section, we mainly emphasize what happens at larger $\varepsilon$, especially near and after the crossing between the 0↓ LL of the X-valley (X0↓) and the 1↓ LL of the Y-valley (Y1↓).

Figure S8 summarizes the evolution of the resistances $R_{xx}$ and $R_{yy}$ at $\nu = 3/2$ as a function of $\varepsilon$. Near $\varepsilon = 0$, magneto-transport is isotropic at $\nu = 3/2$ (Fig. S7(a)). As we apply $\varepsilon$, near $\varepsilon = 1.20 \times 10^{-4}$ (Fig. S7(e)), there

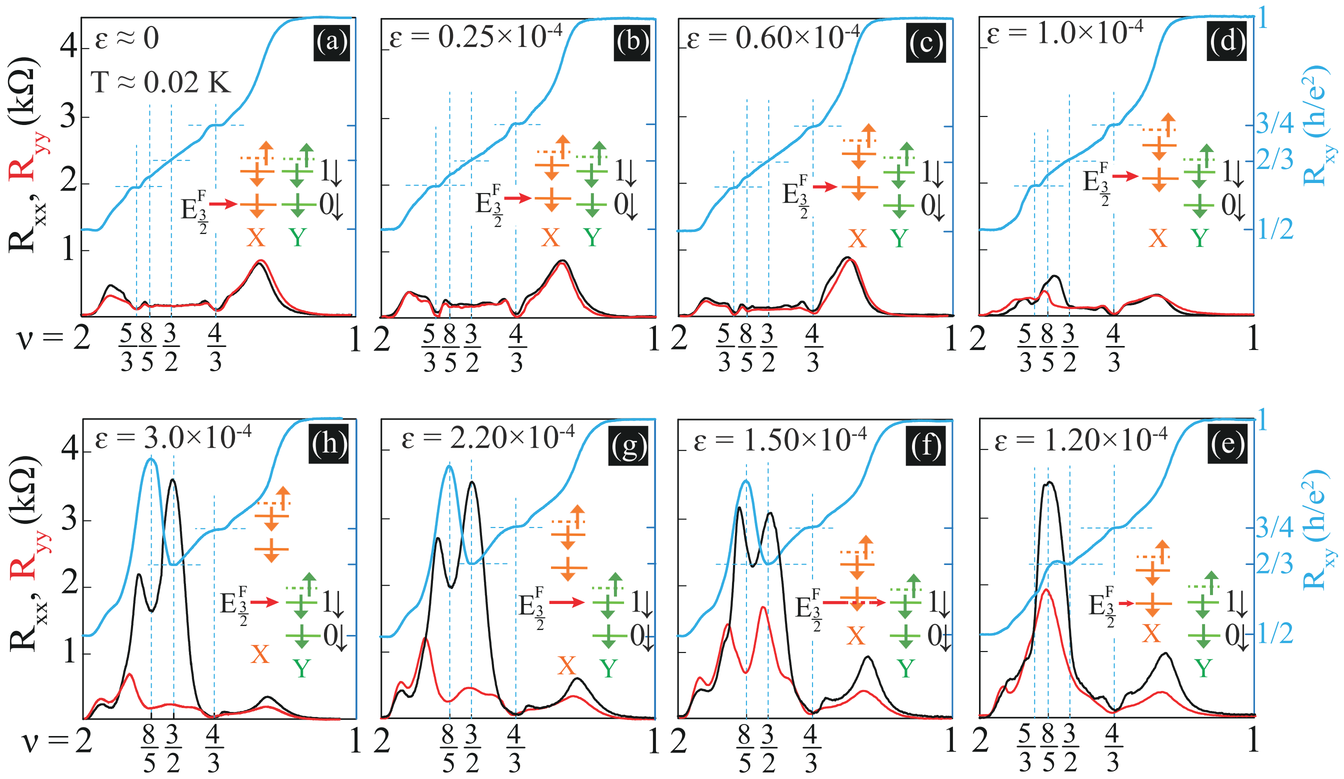

FIG. S7. Evolution of magneto-transport with $\varepsilon$ shown for $2 > \nu > 1$ as the valley occupancy is tuned from both X and Y ($\varepsilon \simeq 0$) to only Y valley ($\varepsilon = 3.0 \times 10^{-4}$). Insets show the corresponding LL diagrams.

is a crossing between the X0↓ and Y1↓ LLs at $\nu = 3/2$. Note that using our measured valley susceptibility (described in Section III), we can estimate the value of $\varepsilon$ required for such a crossing, i.e. $E_V = E_C$, at $\nu = 3/2$. We obtain $\varepsilon \simeq \pm 1.20 \times 10^{-4}$ which is consistent with our observation.

After the LL crossing, the anisotropic phase with a quantized Hall plateau at $\nu = 3/2$, and the unconventional bubble phase at $\nu = 8/5$ start to emerge and become more developed as the gap between the Y1↓ and the nearest LL increases (Fig. S7(g)-(h)). We remark that, above $\varepsilon = 2.20 \times 10^{-4}$, with the increase in $\varepsilon$, we observe no evidence for further phase transitions up to our highest $\varepsilon$. This is also clear from Fig. S8 where we observe a saturation in both $R_{xx}$ and $R_{yy}$ at $\nu = 3/2$ for $|\varepsilon| > 2.20 \times 10^{-4}$. In order to emphasize that at $|\varepsilon| = 3.0 \times 10^{-4}$, the electrons are deep in one valley and $\nu = 3/2$ is firmly in the $N = 1$ LL, we show in Fig. S9 the magneto-resistance at $\varepsilon = -3.0, -2.25$, and $-1.85 \times 10^{-4}$ for comparison. It is clear from the plots that there is almost no change in the traces as more negative strain is applied.

To summarize, we observe a well-quantized $\nu = 3/2$ Hall plateau only when we are past the crossing between the 0↓ and 1↓ LLs and $E^F$ is firmly in the 1↓ LL. We add that, the evolution we observe is different from what is seen in the case of ZnO 2DESs [11]. In ZnO 2DESs, the $\nu = 3/2$ FQHS appears near the crossing between the $N = 0$ and 1 LLs and gives way to an insulating phase when firmly in the $N = 1$ LL. More recently, it was reported that in ZnO 2DESs, there are different phases (in-

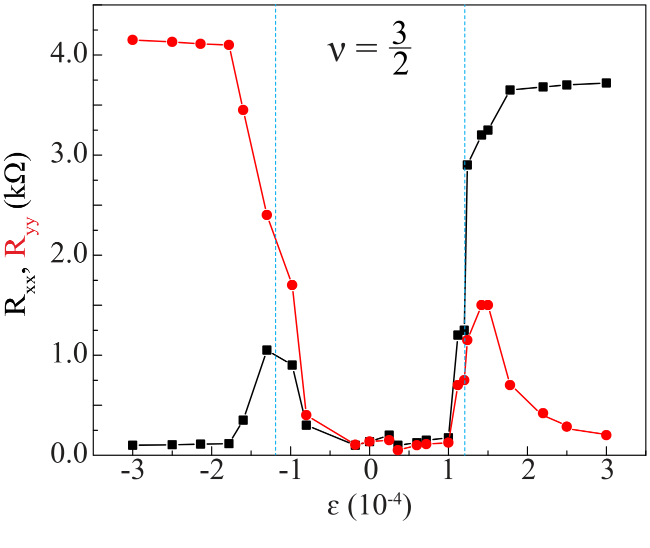

FIG. S8. Magneto-resistance values at $\nu = 3/2$ plotted against $\varepsilon$ at $T \simeq 0.02$ K, summarizing the evolution from a composite Fermi liquid to anisotropic FQHS. The dashed lines mark the approximate strain positions of LL crossing.

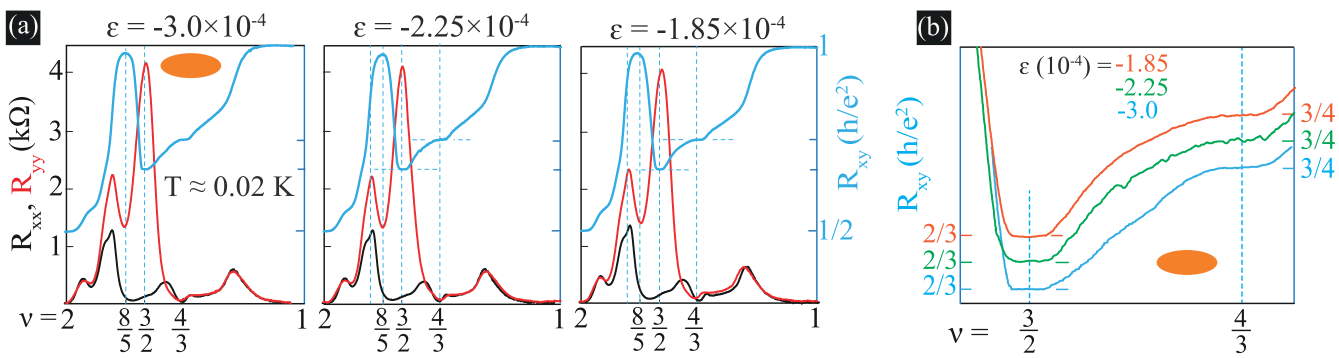


FIG. S9. Magneto-transport at the extreme negative values of strain. (a) $R_{xx}$ (black), $R_{yy}$ (Red) and $R_{xy}$ (blue) traces taken at $T \simeq 0.05$ K showing almost no change in transport when large $\varepsilon$ are applied. (b) Zoomed-in $R_{xy}$ traces for the same $\varepsilon$ as in (a) indicating the presence of a well-quantized Hall plateau at $\nu = 3/2$. These traces corroborate the fact that there is no further phase transition up to our highest $\varepsilon$ as the Fermi energy at $\nu = 3/2$ resides firmly in the $N = 1$ LL.

cluding even-denominator FQHSs) near the LL crossings, depending on the mixing between the LLs [12]. However, in our mass anisotropic AlAs 2DESs, in our limited data, we do not observe such phases near the LL crossings. It is also noteworthy that, unlike our AlAs 2DESs, ZnO 2DESs are isotropic.

Another important observation from the traces in Fig. S7 is the asymmetry in magneto-transport between the electron and hole sides of $\nu = 3/2$ in the $N = 1$ LL. Near the LL crossing, at $\varepsilon = 1.20 \times 10^{-4}$ (Fig. S7(e)), the X0↓ and Y1↓ LLs become energetically close and the $\nu = 5/3$ FQHS disappears although the $\nu = 4/3$ exhibits a reasonably strong FQHS. After the LL crossing, the $\nu = 4/3$ FQHS remains strong, but we do not observe any signature of a FQHS at $\nu = 5/3$. This is in stark contrast to the case of the $N = 0$ LL where we observe well-developed FQHSs at both $\nu = 5/3$ and 4/3 (Fig. S7(a)-(c)). This suggests a breakdown of particle-hole symmetry in the $N = 1$ LL of our 2DES.

## VI. MAGNETO-TRANSPORT AT VERY HIGH $B_\perp$ IN THE $N = 0$ LANDAU LEVEL

The Fermi contour of electrons occupying a single in-plane valley in an AlAs 2DES is intrinsically anisotropic. This results in anisotropic resistances almost everywhere in the magneto-transport traces when X or Y valley is occupied. Intuitively, one would expect that the higher resistance should be along the direction of the larger mass. This is indeed the case for $B = 0$ (Figs. 1(b) and S6) and $\nu > 2$ (Fig. 2). However, as discussed in the main text, the anisotropy is reversed in the range $2 > \nu > 1$ when the anisotropic FQHS emerges. In this section, for a complete understanding of the anisotropic magneto-transport in our AlAs sample, we present magneto-resistance data (Fig. S10) in the extreme quantum limit ($\nu < 1$). These traces were taken in the NHMFL's hybrid magnet.

When the electrons occupy both X and Y valleys, $R_{xx}$ and $R_{yy}$ are essentially isotropic near $\nu = 1/2$ (Fig. S10(b)), similar to the case of $B = 0$ (Figs. 1(b) and S6). This similarity continues when the electrons occupy only one valley. When electrons occupy only the X valley, $R_{xx} > R_{yy}$ near $\nu = 1/2$ (Fig. S10(a)), and vice versa for the Y valley (Fig. S10(c)). This observation is particularly important as it clearly shows that, beyond $2 > \nu > 1$, the anisotropy reverses again and follows the direction of anisotropy at $B = 0$.

## VII. PREVIOUS REPORTS OF ANISOTROPY IN THE $N = 1$ LANDAU LEVEL

The role of anisotropy on the stability of FQHSs and other many-body states of 2DESs has in fact been a subject of great interest lately [13–29]. The FQHSs in the ground ($N = 0$) LL are reported to be reasonably robust in the presence of mass anisotropy [15, 21]. Although the Fermi contour anisotropy makes the composite fermion Fermi sea anisotropic [21], it barely affects the surrounding FQHSs; this is true even for a factor of $\simeq 3.3$ anisotropy in the zero-field Fermi wave-vector [21]. In our measurements of the $N = 0$ LL (see Fig. S10), we also find that, the same FQHS sequences emerge for both isotropic bi-valley and anisotropic single-valley cases. In sharp contrast to the $N = 0$ LL, many-body phases in the first excited ($N = 1$) LL exhibit dramatic changes in response to the Fermi contour anisotropy which is a key finding of our experiments and described in detail in the main text.

Here we discuss briefly some of the other anisotropic phases observed in the $N = 1$ LL which are relevant to our study. In the $N = 1$ LL there is a close competition between the uniform-density FQHSs and the density-modulated nematic phases [22–33]. For example, when a small parallel magnetic field ($B_{||}$) is applied

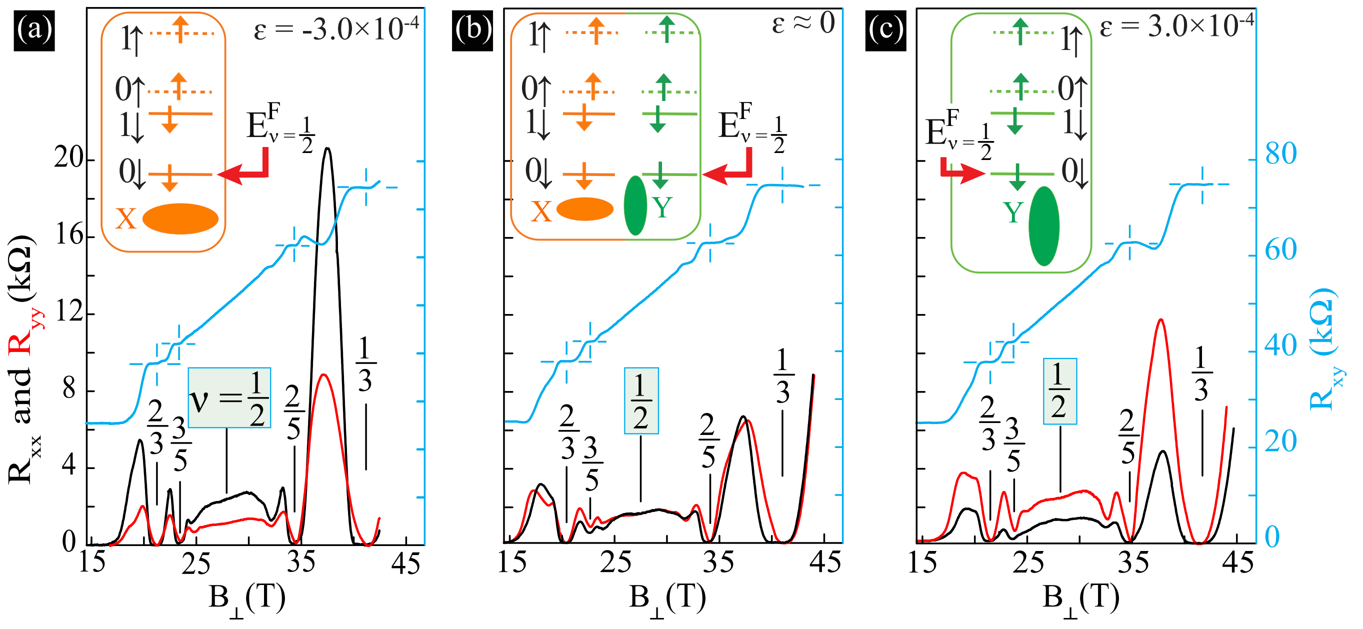


FIG. S10. Magneto-transport in the extreme quantum limit measured using a 45 T hybrid magnet equipped with a dilution fridge with base temperature around $T \simeq 0.05$ K. Presented are the $R_{xx}$ (black), $R_{yy}$ (Red) and $R_{xy}$ (blue) traces when electrons occupy (a) only X valley, (b) both X and Y valleys, and (c) only Y valley. The field positions of the odd-denominator FQHS sequences surrounding the composite fermion Fermi sea at $\nu = 1/2$ are marked with black perpendicular lines. The blue horizontal lines mark the expected quantized values for the corresponding Hall resistances. Corresponding LL diagrams are shown in the insets. The red arrows indicate the Fermi energy at $\nu = 1/2$ for different valley occupancies.

along the x-direction, the $\nu = 7/3$ FQHS in GaAs 2DESs turns to an anisotropic FQHS [24]. An intriguing property of the observed anisotropic $\nu = 7/3$ FQHS is that, below a critical temperature, $R_{xx}$ starts to increase when the temperature is further lowered, while $R_{yy}$ continues to decrease as the temperature approaches zero. These measurements motivated theoretical calculations which discuss the possibility of a transition to an anisotropic, nematic FQHS below a critical temperature at $\nu = 7/3$ in the presence of a small $B_{||}$ [26–28]. These theories, however, predict that below the critical temperature, both $R_{xx}$ and $R_{yy}$ should decrease and ultimately tend to zero as temperature approaches zero; this is different from the experimental observations in Ref. [24] which reveal that $R_{xx}$ increases down to the lowest achieved temperature.

In GaAs 2DESs, another $N = 1$ FQHS, namely the $\nu = 5/2$ FQHS, also turns to an anisotropic nematic FQHS in the presence of a small $B_{||}$ [25]. In this case, consistent with the theoretical expectation for a nematic FQHS [26, 27], both $R_{xx}$ and $R_{yy}$ decrease when the temperature is lowered. However, no finite-temperature transition was observed. Lastly, at larger $B_{||}$, the nematic FQHSs disappear and a compressible nematic phase emerges with its charge density modulated along the direction of $B_{||}$ [22, 23].

Another 2D carrier system, namely the 2D hole system (2DHS) in GaAs exhibits *compressible* anisotropic phases at even-denominator fillings as small as 5/2 even when no $B_{||}$ is applied [30, 31]. (Note that $\nu = 5/2$ would normally correspond to a half-filled $N = 1$ LL, but one should be cautious as the LLs in 2DHSs are non-linear and there are complex LL crossings as a function of perpendicular magnetic filed [34].) It has also been reported that the application of in-plane strain to the 2DHS affects the orientation of the compressible anisotropic phases [32]. The emergence of an anisotropic phase instead of a FQHS has been attributed to the spin-orbit interaction present in the 2DHS [30–32]. However, the application of in-plane strain to the 2DHS also leads to an anisotropic Fermi contour [21]. Considering the orientation of the Fermi contour anisotropy reported in Ref. [21], the directions of the transport anisotropies observed in Ref. [32] are indeed consistent with the directions we observe in our work, namely, the hard axis is along the smaller Fermi wave vector. We emphasize, however, that no quantized Hall resistance was reported for the strained 2DHS [32], or in Refs. [30, 31].

More recently, the isotropic $\nu = 5/2$ FQHS in a GaAs 2DES was reported to undergo a phase transition to a compressible, anisotropic nematic phase in the presence of hydrostatic pressure [33]. This transition has been attributed to a possible Pomeranchuk instability of the composite fermion Fermi liquid [29, 35], although very recent measurements suggest that parameters other than pressure might be playing an important role also [36].

Finally, we add that, the temperature dependence of

the longitudinal resistances we observe at $\nu = 3/2$ share some similarities with the recent data at $\nu = 9/2$ and $11/2$ ($N = 2$ LL) in a GaAs 2DES [37]. Similar to our data, at $\nu = 9/2$ and $11/2$, below a critical temperature, the hard-axis resistance also decreases as the temperature is lowered. This behavior was attributed to a possible nematic to smectic phase transition [37]. However, note that both these phases are expected to be compressible in the $N = 2$ LL and indeed, in stark contrast to our data, no quantized Hall plateau was observed at $\nu = 9/2$ and $11/2$. (In the $N = 2$ LL, a charge density wave ordering is preferred because of the dominance of the exchange energy.) Furthermore, there is no mass anisotropy present in GaAs 2DESs.


[1] E. P. De Poortere, Y. P. Shkolnikov, E. Tutuc, S. J. Papadakis, and M. Shayegan, Enhanced electron mobility and high order fractional quantum Hall states in AlAs quantum wells, Appl. Phys. Lett. **80**, 1583 (2002).

[2] M. Shayegan, E. P. De Poortere, O. Gunawan, Y. P. Shkolnikov, E. Tutuc, and K. Vakili, Two-dimensional electrons occupying multiple valleys in AlAs, Phys. Stat. Sol. (b) **243**, 3629 (2006).

[3] Y. J. Chung, K. W. Baldwin, K. W. West, D. Kamburov, M. Shayegan, and L. N. Pfeiffer, Design rules for modulation-doped AlAs quantum wells, Phys. Rev. Materials **1**, 021002 (2017).

[4] Y. J. Chung, K. A. Villegas Rosales, H. Deng, K. W. Baldwin, K. W. West, M. Shayegan, and L. N. Pfeiffer, Multivalley two-dimensional electron system in an AlAs quantum well with mobility exceeding $2 \times 10^6$ cm$^2$/Vs, Phys. Rev. Materials **2**, 071001(R) (2018).

[5] M. Shayegan, K. Karrai, Y. P. Shkolnikov, K. Vakili, E. P. De Poortere, and S. Manus, Low-temperature, in situ tunable, uniaxial stress measurements in semiconductors using a piezoelectric actuator, Appl. Phys. Lett. **83**, 5235 (2003).

[6] K. Vakili, Y. P. Shkolnikov, E. Tutuc, E. P. De Poortere, and M. Shayegan, Spin susceptibility of two-dimensional electrons in narrow AlAs quantum wells, Phys. Rev. Lett. **92**, 226401 (2004).

[7] T. Gokmen, M. Padmanabhan, and M. Shayegan, Contrast between spin and valley degrees of freedom, Phys. Rev. B **81**, 235305 (2010).

[8] O. Gunawan, Y. P. Shkolnikov, K. Vakili, T. Gokmen, E. P. De Poortere, and M. Shayegan, Valley susceptibility of an interacting two-dimensional electron system, Phys. Rev. Lett. **97**, 186404 (2006).

[9] N. C. Bishop, M. Padmanabhan, K. Vakili, Y. P. Shkolnikov, E. P. De Poortere, and M. Shayegan, Valley polarization and susceptibility of composite fermions around a filling factor $\nu = 3/2$, Phys. Rev. Lett. **98**, 266404 (2007).

[10] M. Padmanabhan, T. Gokmen, and M. Shayegan, Density dependence of valley polarization energy for composite fermions, Phys. Rev. B **80**, 035423 (2009).

[11] J. Falson, D. Maryenko, B. Friess, D. Zhang, Y. Kozuka, A. Tsukazaki, J. H. Smet, and M. Kawasaki, Even-denominator fractional quantum Hall physics in ZnO, Nature Physics **11**, 347 (2015).

[12] J. Falson, D. Tabrea, D. Zhang, I. Sodemann, Y. Kozuka, A. Tsukazaki, M. Kawasaki, K. V. Klitzing and J. H. Smet, A cascade of phase transitions in an orbitally mixed half-filled Landau level, Science Advances **4**, eaat8742 (2018).

[13] T. Gokmen, Medini Padmanabhan, and M. Shayegan, Transference of transport anisotropy to composite fermions, Nature Physics **6**, 621 (2010).

[14] F. D. M. Haldane, Geometrical Description of the Fractional Quantum Hall Effect, Phys. Rev. Lett. **107**, 116801 (2011).

[15] B. Yang, Z. Papić, E. H. Rezayi, R. N. Bhatt, and F. D. M. Haldane, Band mass anisotropy and the intrinsic metric of fractional quantum Hall systems, Phys. Rev. B **85**, 165318 (2012).

[16] H. Wang, R. Narayanan, X. Wan, and F. Zhang, Fractional quantum Hall states in two-dimensional electron systems with anisotropic interactions, Phys. Rev. B **86**, 035122 (2012).

[17] D. A. Abanin, S. A. Parameswaran, S. A. Kivelson, S. L. Sondhi, Nematic valley ordering in quantum Hall systems, Phys. Rev. B **82**, 035428 (2010).

[18] D. Kamburov, Y. Liu, M. Shayegan, L. N. Pfeiffer, K. W. West, and K. W. Baldwin, Composite fermions with tunable Fermi contour anisotropy, Phys. Rev. Lett. **110**, 206801 (2013).

[19] D. Kamburov, M. A. Mueed, M. Shayegan, L. N. Pfeiffer, K. W. West, K. W. Baldwin, J. J. D. Lee, and R. Winkler, Fermi contour anisotropy of GaAs electron-flux composite fermions in parallel magnetic fields, Phys. Rev. B **89**, 085304 (2014).

[20] B. E. Feldman, M. T. Randeria, A. Gyenis, F. Wu, H. Ji, R. J. Cava, A. H. MacDonald, and A. Yazdani, Observation of a nematic quantum Hall liquid on the surface of bismuth, Science **354**, 316 (2016).

[21] I. Jo, K. A. Villegas Rosales, M. A. Mueed, L. N. Pfeiffer, K. W. West, K. W. Baldwin, R. Winkler, M. Padmanabhan, and M. Shayegan, Transference of Fermi contour anisotropy to composite fermions, Phys. Rev. Lett. **119**, 016402 (2017).

[22] M. P. Lilly, K. B. Cooper, J. P. Eisenstein, L. N. Pfeiffer, and K. W. West, Anisotropic states of two-dimensional electron systems in high Landau levels: effect of an in-plane magnetic field, Phys. Rev. Lett. **83**, 824 (1999).

[23] W. Pan, R. R. Du, H. L. Stormer, D. C. Tsui, L. N. Pfeiffer, K. W. Baldwin, and K. W. West, Strongly anisotropic electronic transport at Landau level filling factor $\nu = 9/2$ and $\nu = 5/2$ under a tilted magnetic field, Phys. Rev. Lett. **83**, 820 (1999).

[24] J. Xia, J. P. Eisenstein, L. N. Pfeiffer, and K. W. West, Evidence for a fractionally quantized Hall state with anisotropic longitudinal transport, Nature Physics **7**, 845848 (2011).

[25] Y. Liu, S. Hasdemir, M. Shayegan, L. N. Pfeiffer, K. W. West, and K. W. Baldwin, Evidence for a $\nu = 5/2$ fractional quantum Hall nematic state in parallel magnetic fields, Phys. Rev. B **88**, 035307 (2013).

[26] M. Mulligan, C. Nayak, and S. Kachru, Effective field theory of fractional quantized Hall nematics, Phys. Rev. B **84**, 195124 (2011).

[27] J. Maciejko, B. Hsu, S. A. Kivelson, Y. Park, and S. L. Sondhi, Field theory of the quantum Hall nematic transition, Phys. Rev. B **88**, 125137 (2013).

[28] R. Regnault, J. Maciejko, S. A. Kivelson, and S. L. Sondhi, Evidence of a fractional quantum Hall nematic phase in a microscopic model, Phys. Rev. B **96**, 035150 (2017).

[29] K. Lee, J. Shao, E. A. Kim, F. D. M. Haldane, and E. H. Rezayi, Pomeranchuk instability of composite Fermi liquids, Phys. Rev. Lett. **121**, 147601 (2018).

[30] M. Shayegan, H. C. Manoharan, S. J. Papadakis, and E. P. De Poortere, Anisotropic transport of two-dimensional holes in high Landau levels, Physica E **6**, 40 (2000).

[31] M. J. Manfra, R. de Picciotto, Z. Jiang, S. H. Simon, L. N. Pfeiffer, K. W. West, and A. M. Sergent, Impact of spin-orbit coupling on quantum Hall nematic phases, Phys. Rev. Lett. **98**, 206804 (2007).

[32] S. P. Koduvayur, Y. Lyanda-Geller, S. Khlebnikov, G. Csáthy, M.J. Manfra, L. N. Pfeiffer, K.W. West, and L.P. Rokhinson, Effect of strain on stripe phases in the quantum Hall regime, Phys. Rev. Lett. **106**, 016804 (2011).

[33] N. Samkharadze, K. A. Schreiber, G. C. Gardner, M. J. Manfra, E. Fradkin, and G. A. Csáthy, Observation of a transition from a topologically ordered to a spontaneously broken symmetry phase, Nat. Phys. **12**, 191 (2016).

[34] R. Winkler, Spin-Orbit Coupling Effects in Two-Dimensional Electron and Hole Systems (Springer, Berlin, 2003).

[35] Y. You, G. Y. Cho, and E. Fradkin, Nematic quantum phase transition of composite Fermi liquids in half-filled Landau levels and their geometric response, Phys. Rev. B **93**, 205401 (2016).

[36] K. A. Schreiber, N. Samkharadze, G. C. Gardner, Y. Lyanda-Geller, M. J. Manfra, L. N. Pfeiffer, K. W. West, and G. A. Csáthy, Electron-electron interactions and the paired-to-nematic quantum phase transition in the second Landau level, Nature Communications **9**, 2400 (2018).

[37] Q. Qian, J. Nakamura, S. Fallahi, G. C. Gardner and M. J. Manfra, Possible nematic to smectic phase transition in a two-dimensional electron gas at half-filling, Nature Communications **8**, 1536 (2017).
